# Supplementary material for: Spatial Decay and Limits of Quantum Solute-Solvent Interactions
Source: arXiv:2301.09212 ancillary file (2023-03-23)
Supplement: Supplementary file 1 [file SI.pdf]

# Supporting Information for “Spatial Decay and Limits of Quantum Solute-Solvent Interactions”

Guorong Weng,<sup>†</sup> Amanda Pang,<sup>†,¶</sup> and Vojtěch Vlček<sup>\*,†,‡</sup>

<sup>†</sup>*Department of Chemistry and Biochemistry, University of California, Santa Barbara, California, 93106-9510, United States*

<sup>‡</sup>*Materials Department, University of California, Santa Barbara, California, 93106-5050, United States*

<sup>¶</sup>*Current institution: University of Pennsylvania, Philadelphia, 19104, United states*

E-mail: vlcek@ucsb.edu

# Theory and Methodology

This section summarizes the theories involved in the main text and the corresponding computational details. Technical information about the stochastic *GW* approach can be found in refs 1–3. For the fragment-Pipek-Mezey localization, please refer to ref 4 for more details.

## Molecular Dynamics Simulations

Molecular dynamics (MD) simulations are employed to generate snapshots for each solvated systems. Throughout this work, we use the Gromacs 5 package<sup>5</sup> with the generalized Amber force field, AM1-bcc charge method, and three-dimensional (3D) periodic boundary conditions for all MD calculations. The solute molecule, phenol, is structurally relaxed at the MP2/cc-pVDZ using the NWchem package. For the H<sub>2</sub>O case, we employ the TIP4P water model.<sup>6</sup> For the other four organic solvents, we first build the solvent-only systems using their mass-density at room temperature under 1 atmosphere. These systems are then equilibrated using the NVT ensemble. Finally, these solvents with equilibrated geometries are used to solvate the phenol molecule. The solvated systems are treated with the following: energy minimization, NVT equilibrium, NPT equilibrium, and MD simulations at 300 K. All the MD simulations run 10,000,000 relaxation steps with a time interval of 0.0005 ps, resulting in a total simulation time of 5,000 ps. From the MD trajectory of each solvated system, we extract a snapshot every 1,000 ps and obtain five representative system geometries. These five extracted snapshots are further used in the Density Functional Theory (DFT) calculations and many-body calculations.

## Density Functional Theory Calculations

DFT calculations in this work employ a real-space implementation with 3D periodic boundary conditions (for the solvated systems), the PBE exchange-correlation functional,<sup>7</sup> and Troullier-Martines pseudopotentials.<sup>8</sup> The resulting canonical eigenstates are used in the

following orbital localization and many-body calculations. Parameters of the DFT calculations are provided in Table S1-S5. For all the calculations, the plane-wave kinetic energy cut-off is set at  $26 E_h$ .

## Fragment-Pipek-Mezey Localization

Pipek-Mezey (PM) orbital localization is performed on the set of occupied canonical orbitals to obtain the localized electronic subspace. The original PM cost function  $\mathcal{P}$  reads

$$\mathcal{P}(\mathbf{U}) = \sum_{i=1}^{N_s} \sum_{A=1}^{N_A} [Q_{ii}^A(\mathbf{U})]^2 \quad (\text{S1})$$

where  $\mathbf{U}$  is the unitary matrix that transforms the basis,  $N_s$  is the number of states considered in the transformation,  $N_A$  denotes the number of atoms involved in the transformation, and  $Q$  is the atomic partial charge matrix. When  $\mathcal{P}$  is maximized, the corresponding  $\mathbf{U}$  yields the PM localized orbitals. The  $Q$  matrix is computed by

$$Q_{ij}^{A,n} = \int \psi_i^{n*}(\mathbf{r}) w_A(\mathbf{r}) \psi_j^n(\mathbf{r}) d\mathbf{r} \quad (\text{S2})$$

where  $\psi_i^n$  represents the transformed states at the  $n^{\text{th}}$  iteration step of maximization.  $w_A(\mathbf{r})$  in eq (S2) denotes the atomic weight function, for which we employ the real-space partitioning scheme with the Gaussian form.

If all the atoms are included in eqs. (S1) and (S2), the  $\mathcal{P}$  will reach a global maximum, and localized orbitals will be obtained for the whole system. However, the cost of localization depends linearly on the  $N_A$ , and this will suffer from a cost overhead if one is interested only in a single fragment of the system. Herein, we employ the modified  $\mathcal{P}$ , as introduced in ref 4, for orbital localization of a selected fragment. The fragment weight function is defined as

$$F^k(\mathbf{r}) = \sum_i^{N_A^k} w_i^k(\mathbf{r}) \quad (\text{S3})$$

Here,  $F^k(\mathbf{r})$  is the weight function of the  $k^{\text{th}}$  fragment,  $N_A^k$  is the number of atoms constituting the  $k^{\text{th}}$  fragment, and  $w_i^k(\mathbf{r})$  is the atomic weight function of each atom belonging to the  $k^{\text{th}}$  fragment. The  $Q$  matrix for the selected fragment is thus written as

$$Q_{ij}^{k,n} = \int \psi_i^{n*}(\mathbf{r}) F^k(\mathbf{r}) \psi_j^n(\mathbf{r}) d\mathbf{r} \quad (\text{S4})$$

which is in fact a fragment partial charge matrix. The modified PM cost function with the fragment partial charge matrix reads

$$\mathcal{P}'(\mathbf{U}) = \sum_{i=1}^{N'_s} [Q_{ii}^k(\mathbf{U})]^2 \quad (\text{S5})$$

where  $N'_s$  denotes the number of localized states that are being sought on the  $k^{\text{th}}$  fragment. Note that maximization of  $\mathcal{P}'$  leads to only  $N'_s$  states that are localized on the fragment but not maximally-localized on each atom of the fragment. Yet, these  $N'_s$  states are sufficient to define the electronic subspace for the  $k^{\text{th}}$  fragment. If one is interested in the real PM localized orbitals on each atom of the fragment, these  $N'_s$  can be used as input states to maximize the original cost function  $\mathcal{P}$  in eq (S1).

## Stochastic $G_0W_0$ Calculations

In this work, quasiparticle (QP) energies are computed by applying the non-local and dynamical self-energy as a perturbative correction to the DFT eigenvalue. The QP energy reads

$$\varepsilon_j^{QP} = \varepsilon_j^0 + \langle \phi_j | \hat{\Sigma}_X + \hat{\Sigma}_C(\omega = \varepsilon_j^{QP}) - \hat{v}_{xc} | \phi_j \rangle \quad (\text{S6})$$

Here,  $\varepsilon_j^0$  represents the eigenvalue of the eigenstate  $\phi_j$  using the mean-field exchange functional  $\hat{v}_{xc}$ . The non-local exchange interaction  $\hat{\Sigma}_X$  is equivalent to the Fock operator. The frequency-dependent correlation self-energy  $\hat{\Sigma}_C$  is obtained by fourier transforming the time-dependent counterpart.

In the stochastic  $G_0W_0$  formalism, the Green's function ( $G_0$ ) is sampled by a set of random vectors

$$G_0(\mathbf{r}, \mathbf{r}'; t) = -i\{\zeta(\mathbf{r}; t)\bar{\zeta}(\mathbf{r}')\} \quad (\text{S7})$$

where the brackets  $\{\dots\}$  denote averaging over the number of random vectors used in sampling. The random function  $\bar{\zeta}(\mathbf{r})$  is given by

$$\bar{\zeta}(\mathbf{r}) = \pm \frac{1}{dV} \quad (\text{S8})$$

Here,  $dV$  is the unit volume of the real-space grid, and the plus-minus sign represents the randomness. The time-evolved projected random function  $\zeta(\mathbf{r}; t)$  is written as

$$\zeta(\mathbf{r}; t) = \begin{cases} \langle \mathbf{r} | e^{-i\hat{H}_0 t} \hat{P}^{occ} | \bar{\zeta} \rangle & t < 0 \\ \langle \mathbf{r} | e^{-i\hat{H}_0 t} (\hat{I} - \hat{P}^{occ}) | \bar{\zeta} \rangle & t > 0 \end{cases} \quad (\text{S9})$$

In eq (S9),  $\hat{H}_0$  is the static mean-field Hamiltonian used in DFT calculations,  $\hat{P}^{occ}$  is the projector composed of all the occupied states, and  $\hat{I}$  is the identity.

The stochastic form of the  $G_0W_0$  correlation self-energy reads

$$\langle \phi_j | \hat{\Sigma}_C(t) | \phi_j \rangle = \left\{ \int \phi_j(\mathbf{r}) \zeta(\mathbf{r}; t) u(\mathbf{r}; t) d\mathbf{r} \right\} \quad (\text{S10})$$

Here,  $u(\mathbf{r}; t)$  is the time-dependent potential due to the induced charge density. It is derived from the following retarded potential  $\tilde{u}(\mathbf{r}; t)$

$$\tilde{u}(\mathbf{r}; t) = \int \nu(\mathbf{r}, \mathbf{r}') \delta n(\mathbf{r}'; t) d\mathbf{r}' \quad (\text{S11})$$

where  $\nu(\mathbf{r}, \mathbf{r}') = \frac{1}{|\mathbf{r} - \mathbf{r}'|}$  is the Coulomb kernel, and the time-dependent induced charge density fluctuations ( $\delta n(\mathbf{r}; t)$ ) is also sampled by another set of random vectors. Further details of deriving the  $\delta n(\mathbf{r}; t)$  are provided in the next section.

# Generalized Decomposition of *GW* Correlation Self-energy

## Fragment Electronic Subspace

For solute-solvent systems, localized orbitals provide a straightforward and convenient way to separate the solute from the environment. As mentioned above, the set of regionally PM localized orbitals on a specific molecule can be obtained directly by constructing a fragment. Moreover, the localization can be done by sequentially exhausting the orbital space.<sup>4</sup> Here, we first demonstrate the construction of an electronic subspace for the solute molecule, and then generalize it to any fragment in the system.

For the solute molecule, the fragment is defined by the following weight function

$$F^{mol}(\mathbf{r}) = \sum_i^{N_A^{mol}} w_i(\mathbf{r}) \quad (\text{S12})$$

where  $N_A^{mol}$  represents the number of atoms of the molecule and  $w_i(\mathbf{r})$  is the atomic weight function of each atom using the real-space partitioning. This fragment weight function is used in the orbital localization (see eqs. (S4) and (S5)), which leads to regionally localized orbitals. The localization is essentially broken into two steps: (1) search for  $N_s$  localized states on the molecule; (2) localize these  $N_s$  states on each atom of the molecule. This work focuses on the occupied subspace, and  $N_s$  includes all the valence electrons of the molecule. Note that only the second step provides the PM localized orbitals. However, the first step is sufficient to separate the solute from the environment. Mathematically, the molecular electronic subspace is defined by the following projector

$$\hat{P}^{mol} = \sum_i^{N_s} |\psi_i^{mol}\rangle \langle \psi_i^{mol}| \quad (\text{S13})$$

where  $\psi_i^{mol}$  represents a localized orbital on the solute molecule. This set of localized basis

is also used to reconstruct the molecular state  $\phi_j^R$

$$|\phi_j^R\rangle = \sum_i^{N_s} \alpha_{ji} |\psi_i^{mol}\rangle \quad (\text{S14})$$

Here,  $\alpha_{ji}$  is the coefficient obtained from decomposing the  $\phi_j^{iso}$  of the isolated molecule in its localized basis. There is a one-to-one correspondence between the localized basis of the solvated molecule and that of the isolated molecule. The full recipe can be found in our previous work.<sup>9</sup> The superscript “ $R$ ” in eq (S14) is omitted for clarity in this work.

Analogously, we can define a weight function of any fragment in the system for the orbital localization

$$F^k(\mathbf{r}) = \sum_i^{N_A^k} w_i^k(\mathbf{r}) \quad (\text{S15})$$

Here,  $N_A^k$  denotes the number of atoms that constitute the  $k^{\text{th}}$  fragment. In a multi-molecule system, a fragment can be a single molecule or a cluster of molecules. The corresponding electronic subspace is then given by

$$\hat{P}^k = \sum_i^{N'_s} |\psi_i^k\rangle \langle \psi_i^k| \quad (\text{S16})$$

where  $\psi_i^k$  is a localized orbital and  $N'_s$  represents the number of localized occupied orbitals on the  $k^{\text{th}}$  fragment.

In our solute-solvent systems, we first separate the solute molecule from the solvent environment, and then fragment the environment into multiple solvent shells. The solvent molecules within the same shell are (ideally) of the same distance away from the solute. The shell weight function  $F_s^k$  has the following form

$$F_s^k(\mathbf{r}; \mathbf{R}^k) = \sum_i^{N_A^k} w_i^k(\mathbf{r}) \quad (\text{S17})$$

Here, the  $k^{\text{th}}$  shell is characterized by the distance  $\mathbf{R}^k$ . The shell weight function sums over

all the  $N_A^k$  atoms in the  $k^{\text{th}}$  shell. Accordingly, the electronic subspace of the  $k^{\text{th}}$  shell is defined by the projector in eq S16.

## Fragment Correlation Self-energy

The frequency-dependent correlation self-energy  $\hat{\Sigma}_C(\omega)$  in eq (S6) is practically obtained from the Fourier transformation of the time-dependent counterpart  $\hat{\Sigma}_C(t)$  (eq (S10)). In the *GW* approximation, the  $\Sigma_C(t)$  (expectation value) stems from the time-dependent charge density fluctuations  $\delta n(t)$  (see eqs. (S10) and (S11)) induced by the electron removal/addition

$$\Sigma_C(t) = \Sigma_C[\delta n(t), t] \quad (\text{S18})$$

In a real-time and real-space implementation,  $\delta n(t)$  is computed by

$$\delta n(\mathbf{r}, t) = n(\mathbf{r}, t) - n_0(\mathbf{r}) \quad (\text{S19})$$

where  $n(\mathbf{r}, t)$  is computed from the time-evolved single-particle states and  $n_0(\mathbf{r})$  denotes the ground-state (GS) density. The deterministic  $n_0(\mathbf{r})$  is usually obtained from all the  $N_{occ}$  occupied canonical KS orbitals

$$n_0(\mathbf{r}) = \sum_i^{N_{occ}} \phi_i^*(\mathbf{r}) \phi_i(\mathbf{r}) \quad (\text{S20})$$

Alternatively, the GS density can also be expressed by a set of unitary transformed states, e.g., localized orbitals

$$n_0(\mathbf{r}) = \sum_i^{N_{occ}} \psi_i^*(\mathbf{r}) \psi_i(\mathbf{r}) \quad (\text{S21})$$

where  $\psi_i$  represents a localized orbital. Upon the fragmentation of a system, the GS density can be further written as

$$n_0(\mathbf{r}) = \sum_k^{N_{frag}} \sum_i^{N_{occ}^k} \psi_i^{k*}(\mathbf{r}) \psi_i^k(\mathbf{r}) = \sum_k^{N_{frag}} n_0^k(\mathbf{r}) \quad (\text{S22})$$

Here,  $N_{occ}^k$  is the number of occupied states on the  $k^{\text{th}}$  fragment.  $\psi_i^k$  and  $n_0^k(\mathbf{r})$  denote an orbital and the density localized on the  $k^{\text{th}}$  fragment, respectively.

In contrast to  $n_0(\mathbf{r})$ , the time-dependent density  $n(\mathbf{r}, t)$  is calculated by a set of time-evolved states that are perturbed by the electron addition/removal at  $t = 0$ . In order to express  $n(\mathbf{r}, t)$  in the same form of eq (S22), we make the following assumption in this work: the perturbed and time-evolved  $\psi^k$  stay localized on the  $k^{\text{th}}$  fragment. In other words, we assume no intermolecular charge transfer happens and all the density fluctuations remain on the fragment. This “local density fluctuations” assumption is reasonable when there is no apparent donor-acceptor character found in a van-der Waals bound molecular system. Upon this assumption,  $n(\mathbf{r}, t)$  is written as

$$n(\mathbf{r}, t) = \sum_k^{N_{frag}} \sum_i^{N_{occ}^k} \psi_i^{k*}(\mathbf{r}, t) \psi_i^k(\mathbf{r}, t) = \sum_k^{N_{frag}} n^k(\mathbf{r}, t) \quad (\text{S23})$$

where  $\psi_i^k$  represents a time-evolved localized orbital on the  $k^{\text{th}}$  fragment, and  $n^k(\mathbf{r}, t)$  is the time-evolved density localized on the  $k^{\text{th}}$  fragment.

Plugging eqs. (S22) and (S23) in Eq (S19), the induced density fluctuation  $\delta n(\mathbf{r}, t)$  is thus fragmented

$$\delta n(\mathbf{r}, t) = \sum_k^{N_{frag}} n^k(\mathbf{r}, t) - \sum_k^{N_{frag}} n_0^k(\mathbf{r}) = \sum_k^{N_{frag}} \delta n^k(\mathbf{r}, t) \quad (\text{S24})$$

where  $\delta n^k(\mathbf{r}, t)$  denotes the local density fluctuation on the  $k^{\text{th}}$  fragment. The fragmented

$\delta n(\mathbf{r}, t)$  further leads to the fragment correlation energy  $\Sigma_C$

$$\Sigma_C[\delta n(t), t] = \sum_k^{N_{frag}} \Sigma_C^k [\delta n^k(\mathbf{r}, t), t] \quad (\text{S25})$$

For a specific molecular state  $\phi_j$ , the fragmentation of  $\Sigma_C$  in the frequency domains reads

$$\Sigma_C(\omega = \varepsilon_j^{QP}) = \sum_k^{N_{frag}} \Sigma_C^k(\omega = \varepsilon_j^{QP}) \quad (\text{S26})$$

In this work, we do not aim to prove the equivalence shown in eq (S26). Instead, we first compute the correlation energy contributed from a specific fragment, e.g., a solvation shell at distance  $\mathbf{R}^k$ , and then study the decay of  $\Sigma_C^k$  as a function of  $\mathbf{R}^k$ .

In our stochastic *GW* formalism, both  $n(\mathbf{r}, t)$  and  $n_0(\mathbf{r})$  are stochastically sampled by a set of random functions, and  $n_0(\mathbf{r})$  also becomes time-dependent due to its stochastic nature

$$n(\mathbf{r}, t) = \{\eta^*(\mathbf{r}, t)\eta(\mathbf{r}, t)\} \quad (\text{S27})$$

At  $t = 0$ ,  $\eta(\mathbf{r})$  is a random vector projected onto the occupied subspace

$$\eta(\mathbf{r}) = \langle \mathbf{r} | \hat{P}^{occ} | \bar{\eta} \rangle \quad (\text{S28})$$

where  $\bar{\eta}$  is a random function in real space:  $\bar{\eta}(\mathbf{r}) = \pm \frac{1}{\text{dV}}$  (dV is the unit volume). The stochastic resolution of identity is satisfied by the constructed  $\bar{\eta}$ .<sup>1,2</sup> The projector  $\hat{P}^{occ}$  consists of all the occupied states. Similar to the deterministic case,  $\eta(\mathbf{r})$  is perturbed at  $t = 0$  by the electron addition/removal and then time-evolved, which gives  $n(\mathbf{r}, t)$  equivalent to the one in eq (S19). Without perturbation, the time-evolved  $\eta$  instead leads to  $n_0(\mathbf{r}, t)$ . And the induced density fluctuation  $\delta n(\mathbf{r}, t)$  is then generated via eq (S19) using the stochastic  $n(\mathbf{r}, t)$  and  $n_0(\mathbf{r}, t)$

$$\delta n(\mathbf{r}, t) = n(\mathbf{r}, t) - n_0(\mathbf{r}, t) \quad (\text{S29})$$

In the previous section, we introduce the electronic subspace for the  $k^{\text{th}}$  solvation shell. The stochastic sampling of  $\delta n^k(\mathbf{r}, t)$  in eq (S24) can be achieved by replacing the operator  $\hat{P}^{occ}$  in eq S28 with  $\hat{P}^k$  (eq S16)

$$\eta^k(\mathbf{r}) = \langle \mathbf{r} | \hat{P}^k | \bar{\eta} \rangle \quad (\text{S30})$$

Here,  $\eta^k(\mathbf{r})$  represents a localized random function on the  $k^{\text{th}}$  solvation shell.  $\delta n^k(\mathbf{r}, t)$  can then be readily calculated by using  $\eta^k(\mathbf{r})$  in eqs. (S27) and (S29). Finally, the correlation energy contributed from the  $k^{\text{th}}$  solvation shell is computed by the  $\delta n^k(\mathbf{r}, t)$ . Again, the stochastic implementation can easily treat any fragment with up to thousands of electrons. In the Results and Discussion section of the main text, we demonstrate the  $\mathbf{R}^k$ -dependence of  $\Sigma_C$ .

## Supplementary Tables and Figures

**Table S1: Parameters of the simulation box used in DFT calculations for the H<sub>2</sub>O solvated system. All lengths are provided in Bohr unit.**

| snapshot | small cell       |              |                 | large cell       |              |                 |
|----------|------------------|--------------|-----------------|------------------|--------------|-----------------|
|          | lattice constant | grid spacing | grid size       | lattice constant | grid spacing | grid size       |
| 1        | 29.663           | 0.3903       | 76 <sup>3</sup> | 38.360           | 0.3996       | 96 <sup>3</sup> |
| 2        | 30.366           | 0.3996       | 76 <sup>3</sup> | 38.868           | 0.4049       | 96 <sup>3</sup> |
| 3        | 29.646           | 0.3901       | 76 <sup>3</sup> | 38.503           | 0.4011       | 96 <sup>3</sup> |
| 4        | 29.982           | 0.3945       | 76 <sup>3</sup> | 38.700           | 0.4031       | 96 <sup>3</sup> |
| 5        | 29.525           | 0.3885       | 76 <sup>3</sup> | 38.915           | 0.4054       | 96 <sup>3</sup> |

**Table S2: Parameters of the simulation box used in DFT calculations for the ACN solvated system. All lengths are provided in Bohr unit.**

| snapshot | small cell       |              |                 | large cell       |              |                 |
|----------|------------------|--------------|-----------------|------------------|--------------|-----------------|
|          | lattice constant | grid spacing | grid size       | lattice constant | grid spacing | grid size       |
| 1        | 26.946           | 0.3963       | 68 <sup>3</sup> | 33.991           | 0.3952       | 86 <sup>3</sup> |
| 2        | 26.473           | 0.3893       | 68 <sup>3</sup> | 34.047           | 0.3959       | 86 <sup>3</sup> |
| 3        | 26.742           | 0.3933       | 68 <sup>3</sup> | 34.215           | 0.3979       | 86 <sup>3</sup> |
| 4        | 27.159           | 0.3994       | 68 <sup>3</sup> | 34.824           | 0.4049       | 86 <sup>3</sup> |
| 5        | 26.566           | 0.3907       | 68 <sup>3</sup> | 34.157           | 0.3972       | 86 <sup>3</sup> |

**Table S3: Parameters of the simulation box used in DFT calculations for the DCM solvated system. All lengths are provided in Bohr unit.**

| snapshot | small cell       |              |                 | large cell       |              |                 |
|----------|------------------|--------------|-----------------|------------------|--------------|-----------------|
|          | lattice constant | grid spacing | grid size       | lattice constant | grid spacing | grid size       |
| 1        | 29.126           | 0.3936       | 74 <sup>3</sup> | 39.257           | 0.4006       | 98 <sup>3</sup> |
| 2        | 29.196           | 0.3945       | 74 <sup>3</sup> | 38.857           | 0.3965       | 98 <sup>3</sup> |
| 3        | 29.051           | 0.3926       | 74 <sup>3</sup> | 38.208           | 0.3899       | 98 <sup>3</sup> |
| 4        | 29.680           | 0.4011       | 74 <sup>3</sup> | 38.460           | 0.3924       | 98 <sup>3</sup> |
| 5        | 29.170           | 0.3942       | 74 <sup>3</sup> | 38.845           | 0.3954       | 98 <sup>3</sup> |

**Table S4: Parameters of the simulation box used in DFT calculations for the THF solvated system. All lengths are provided in Bohr unit.**

| snapshot | small cell       |              |                 | large cell       |              |                 |
|----------|------------------|--------------|-----------------|------------------|--------------|-----------------|
|          | lattice constant | grid spacing | grid size       | lattice constant | grid spacing | grid size       |
| 1        | 30.547           | 0.3916       | 78 <sup>3</sup> | 37.740           | 0.3931       | 96 <sup>3</sup> |
| 2        | 31.103           | 0.3988       | 78 <sup>3</sup> | 37.899           | 0.3948       | 96 <sup>3</sup> |
| 3        | 30.449           | 0.3904       | 78 <sup>3</sup> | 38.129           | 0.3972       | 96 <sup>3</sup> |
| 4        | 30.665           | 0.3931       | 78 <sup>3</sup> | 37.744           | 0.3932       | 96 <sup>3</sup> |
| 5        | 31.124           | 0.3990       | 78 <sup>3</sup> | 37.626           | 0.3919       | 96 <sup>3</sup> |

**Table S5: Parameters of the simulation box used in DFT calculations for the BEN solvated system. All lengths are provided in Bohr unit.**

| snapshot | small cell       |              |                 | large cell       |              |                  |
|----------|------------------|--------------|-----------------|------------------|--------------|------------------|
|          | lattice constant | grid spacing | grid size       | lattice constant | grid spacing | grid size        |
| 1        | 31.868           | 0.3984       | 80 <sup>3</sup> | 40.264           | 0.3947       | 102 <sup>3</sup> |
| 2        | 32.167           | 0.4021       | 80 <sup>3</sup> | 40.822           | 0.4002       | 102 <sup>3</sup> |
| 3        | 31.918           | 0.3990       | 80 <sup>3</sup> | 41.221           | 0.4041       | 102 <sup>3</sup> |
| 4        | 32.386           | 0.4048       | 80 <sup>3</sup> | 40.979           | 0.4018       | 102 <sup>3</sup> |
| 5        | 31.353           | 0.3919       | 80 <sup>3</sup> | 40.452           | 0.3966       | 102 <sup>3</sup> |

**Table S6: Parameters in the *GW* calculations of all systems.**

| Parameters                                                                                                               | value |
|--------------------------------------------------------------------------------------------------------------------------|-------|
| plane wave cut-off (hartree)                                                                                             | 26    |
| number of random vectors used for sparse stochastic compression                                                          | 20000 |
| number of random vectors characterizing the screened Coulomb interaction (per each vector sampling the Green's function) | 16    |
| number of vectors sampling the Green's function                                                                          | 2000  |
| maximum time for real-time propagation of the dynamical self-energy (a.u.)                                               | 50    |

**Table S7:** Number of solvent molecules in the two simulation cells of each solvated system.

| solvent          | small cell | large cell |
|------------------|------------|------------|
| H <sub>2</sub> O | 118        | 273        |
| ACN              | 33         | 64         |
| DCM              | 31         | 73         |
| THF              | 31         | 59         |
| BEN              | 30         | 62         |

**Table S8:** HOMO QP energies of isolated and solvated phenol and the ionization potential (IP) shifts. All energy values are averaged over five snapshots and reported in eV unit. Standard deviations ( $\sigma$ ) are provided in parenthesis. The mean polarizability ( $\alpha_m$ ) of each solvent is provided for comparing the solvation many-body effects.

| solvent          | small cell                           |                                       |                               | large cell                           |                                       |                               | $\alpha_m$ ( $\text{\AA}^3$ ) |
|------------------|--------------------------------------|---------------------------------------|-------------------------------|--------------------------------------|---------------------------------------|-------------------------------|-------------------------------|
|                  | $\epsilon^{\text{iso}}$ ( $\sigma$ ) | $\epsilon^{\text{solv}}$ ( $\sigma$ ) | $\Delta\epsilon$ ( $\sigma$ ) | $\epsilon^{\text{iso}}$ ( $\sigma$ ) | $\epsilon^{\text{solv}}$ ( $\sigma$ ) | $\Delta\epsilon$ ( $\sigma$ ) |                               |
| H <sub>2</sub> O | -8.26 (0.08)                         | -7.34 (0.14)                          | 0.92 (0.06)                   | -8.16 (0.16)                         | -7.11 (0.17)                          | 1.05 (0.06)                   | 1.48                          |
| ACN              | -8.21 (0.07)                         | -7.15 (0.08)                          | 1.06 (0.05)                   | -8.21 (0.15)                         | -7.11 (0.14)                          | 1.10 (0.05)                   | 4.41                          |
| DCM              | -8.42 (0.23)                         | -7.14 (0.27)                          | 1.28 (0.06)                   | -8.18 (0.15)                         | -6.75 (0.14)                          | 1.43 (0.08)                   | 6.50                          |
| THF              | -8.16 (0.09)                         | -7.02 (0.04)                          | 1.14 (0.08)                   | -8.16 (0.07)                         | -6.83 (0.10)                          | 1.33 (0.07)                   | 7.93                          |
| BEN              | -8.18 (0.07)                         | -6.98 (0.07)                          | 1.20 (0.06)                   | -8.22 (0.10)                         | -6.83 (0.14)                          | 1.39 (0.05)                   | 10.38                         |

**Table S9:** Number of *effective* solvent molecules in each snapshot of each solvated system. The results are obtained from the large simulation cells.

| solvent          | snapshot1 | snapshot2 | snapshot3 | snapshot4 | snapshot5 | average |
|------------------|-----------|-----------|-----------|-----------|-----------|---------|
| H <sub>2</sub> O | 99        | 98        | 99        | 90        | 97        | 97      |
| ACN              | 31        | 32        | 31        | 32        | 34        | 32      |
| DCM              | 20        | 25        | 23        | 27        | 24        | 24      |
| THF              | 21        | 18        | 18        | 19        | 20        | 19      |
| BEN              | 18        | 19        | 15        | 15        | 14        | 16      |

**Table S10:** Number of effective solvent molecules and average energy shift per solvent molecule derived from the proposed solvation model. The resulting QP energy shifts are compared with the first-principle results labelled by the superscript 0.

| solvent          | $N_{\text{eff}}^0$ | $\Delta\epsilon^0$ | $N_{\text{eff}}^m$ | $\overline{\Delta\epsilon}^m$ | $N_{\text{eff}}^m \times \overline{\Delta\epsilon}^m$ | $N_{\text{eff}}^0 \times \overline{\Delta\epsilon}^m$ |
|------------------|--------------------|--------------------|--------------------|-------------------------------|-------------------------------------------------------|-------------------------------------------------------|
| H <sub>2</sub> O | 97                 | 1.05               | 96                 | 0.0122                        | 1.16                                                  | 1.17                                                  |
| ACN              | 32                 | 1.10               | 33                 | 0.0374                        | 1.23                                                  | 1.20                                                  |
| DCM              | 24                 | 1.43               | 27                 | 0.0553                        | 1.49                                                  | 1.32                                                  |
| THF              | 19                 | 1.33               | 21                 | 0.0676                        | 1.43                                                  | 1.30                                                  |
| BEN              | 16                 | 1.39               | 19                 | 0.0887                        | 1.73                                                  | 1.44                                                  |

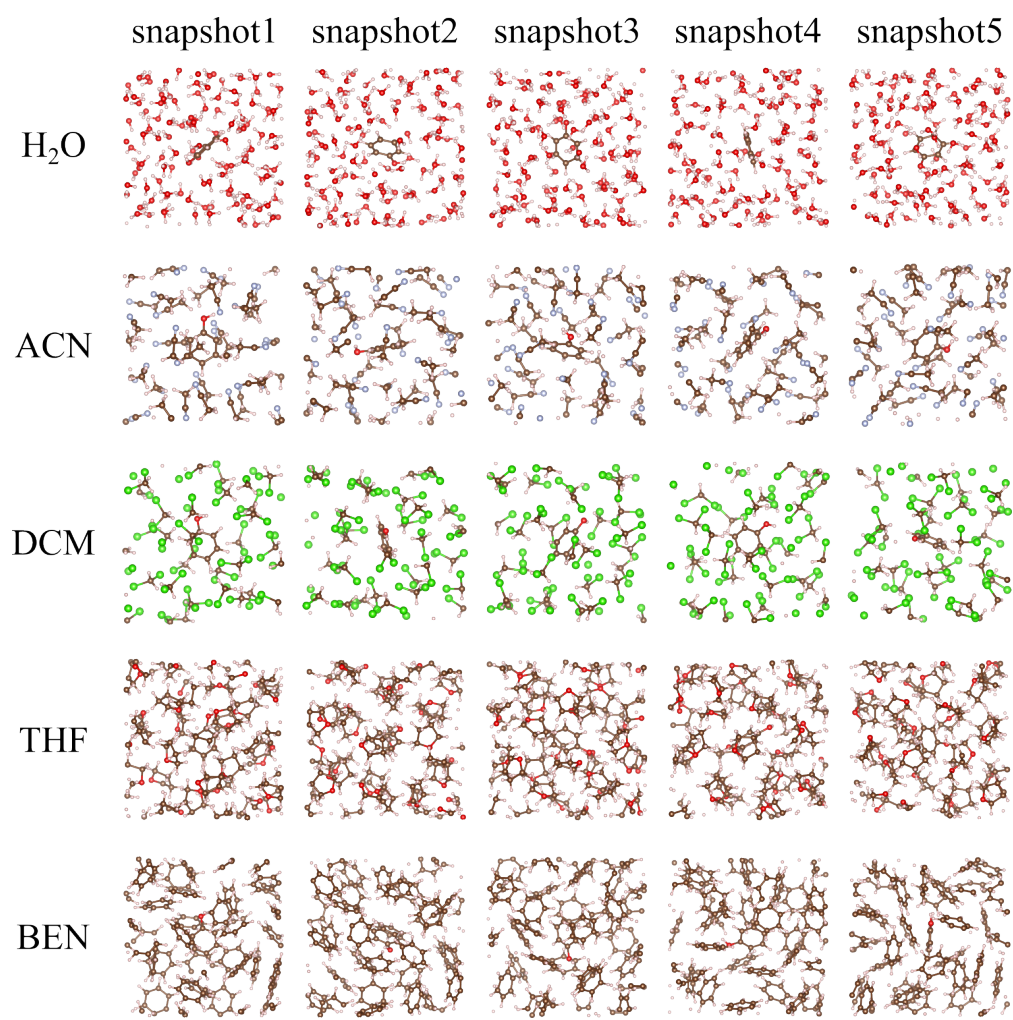

Figure S1: Five extracted snapshots from the MD trajectories of each solvated system using the small simulation cell.

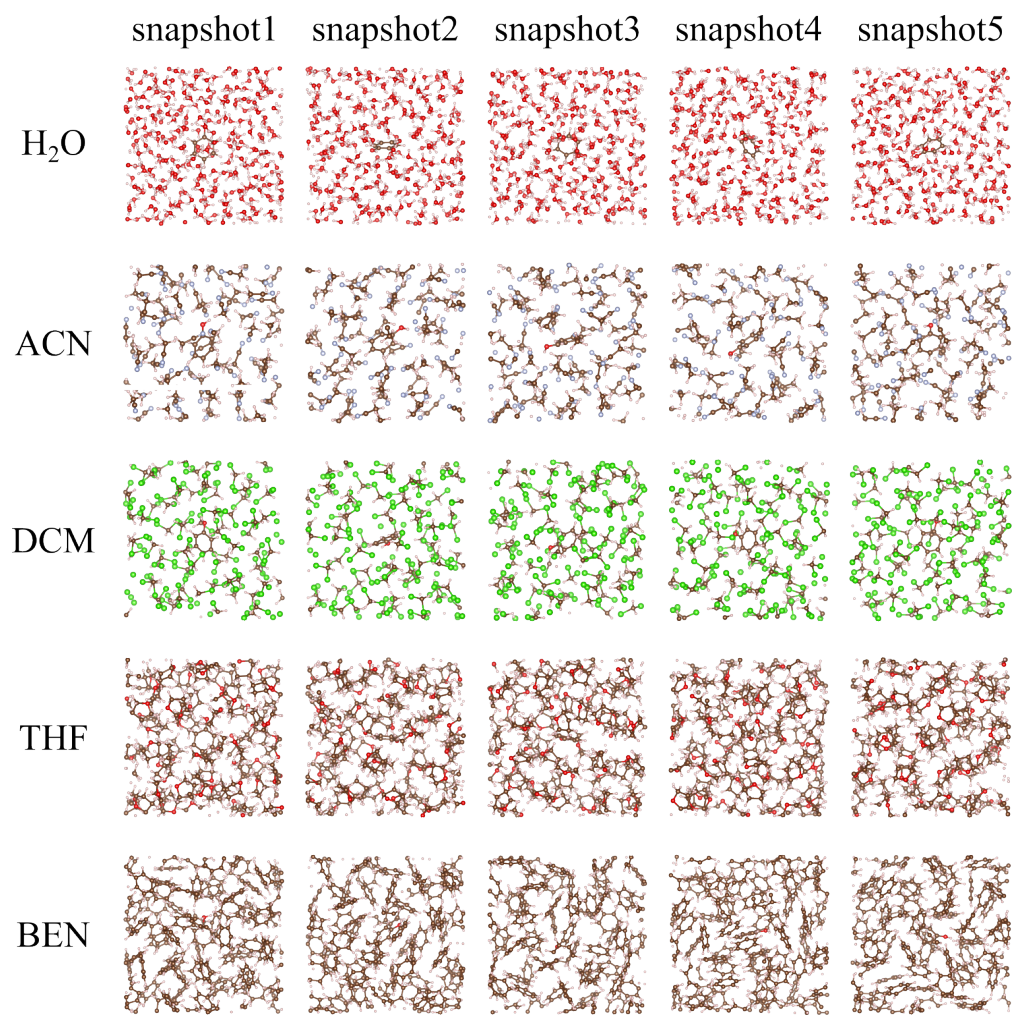

Figure S2: Five extracted snapshots from the MD trajectories of each solvated system using the large simulation cell.

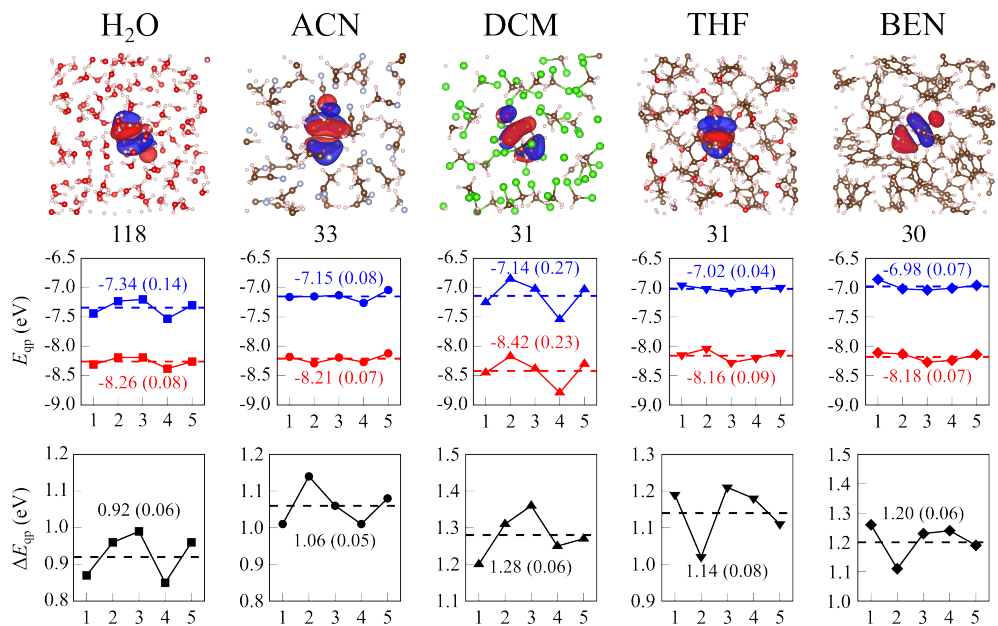

Figure S3: Computational results for each solvated system using the small simulation cell: representative solvated HOMO (upper part), HOMO QP energies of each selected snapshot (middle part), and QP energy shifts between the isolated and solvated HOMO of each selected snapshot (lower part). The blue color represents the solvated HOMO while the red color represents the isolated counterpart. The dashed line indicates the average value over the five snapshots with the standard deviation provided in parenthesis.

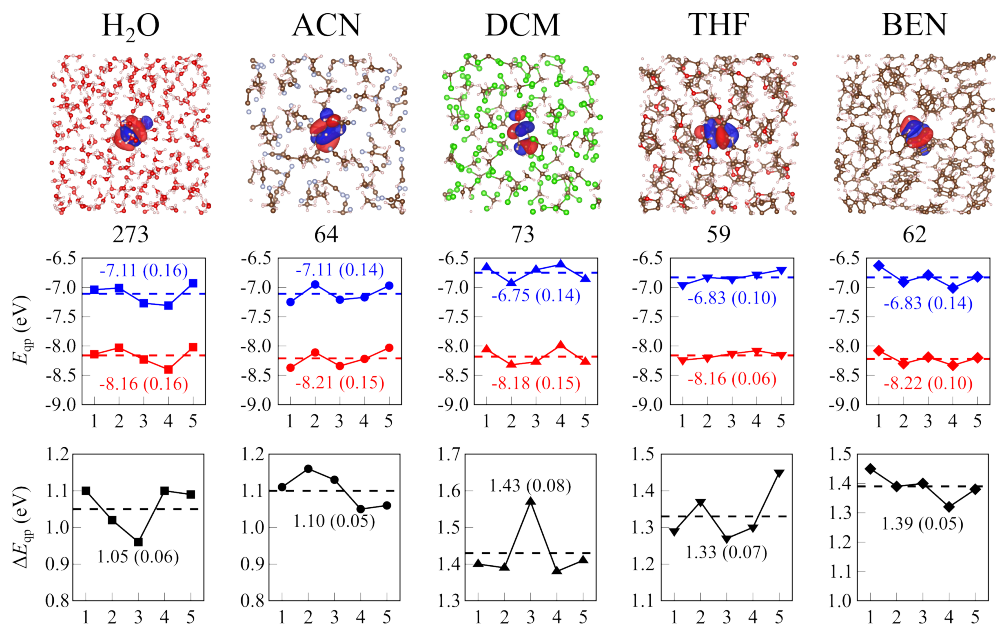

Figure S4: Computational results for each solvated system using the large simulation cell: representative solvated HOMO (upper part), HOMO QP energies of each selected snapshot (middle part), and QP energy shifts between the isolated and solvated HOMO of each selected snapshot (lower part). The blue color represents the solvated HOMO while the red color represents the isolated counterpart. The dashed line indicates the average value over the five snapshots with the standard deviation provided in parenthesis.

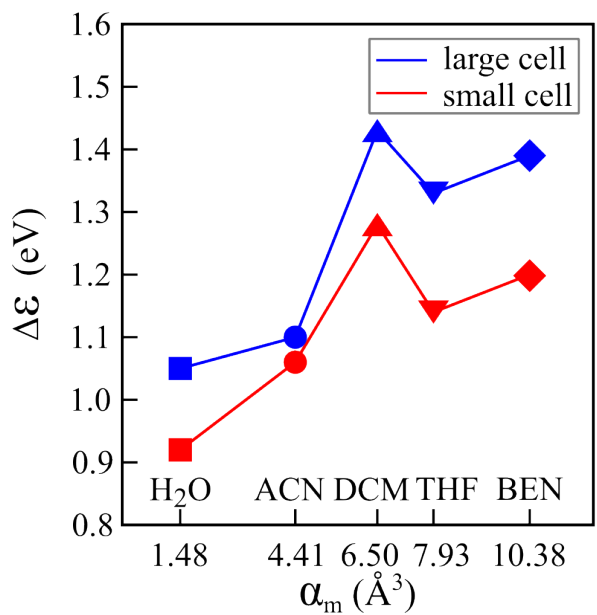

Figure S5: IP shifts  $\Delta\epsilon$  plotted as a function of the mean polarizability; the two colors denote the two simulation cells with different number of solvent molecules.

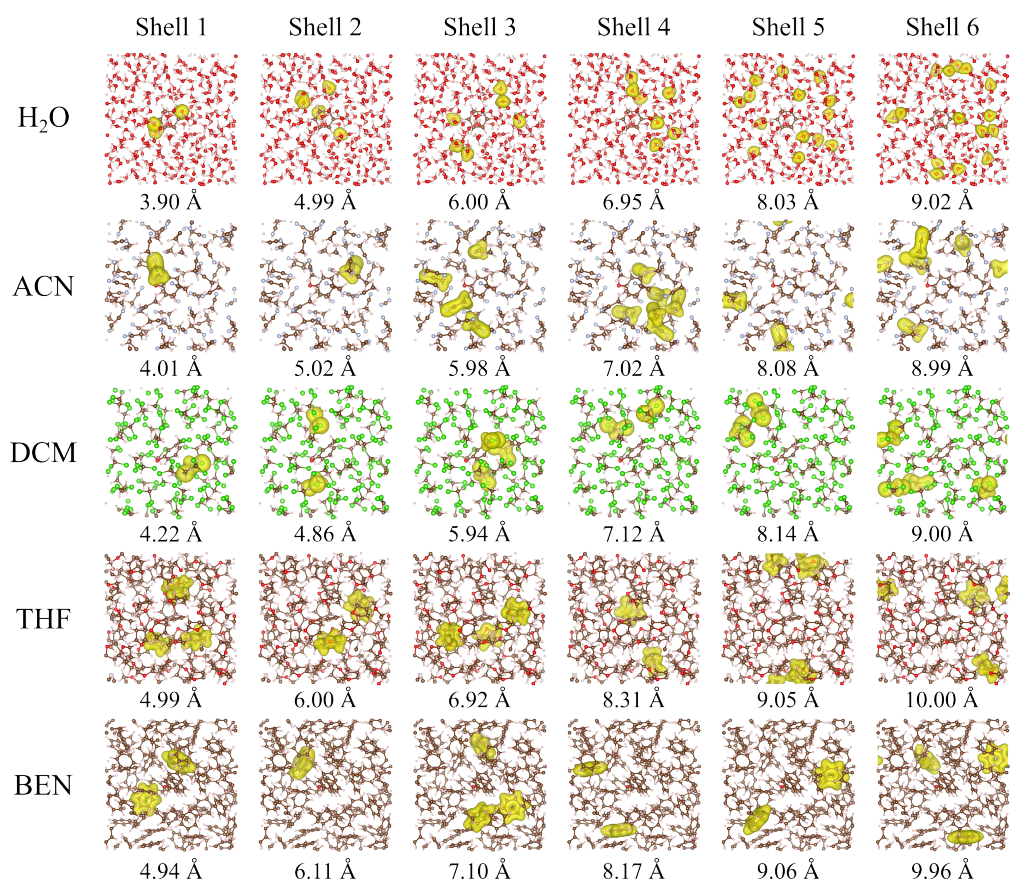

Figure S6: Solvation shells represented by the electron density at six different distances for each solvated system.

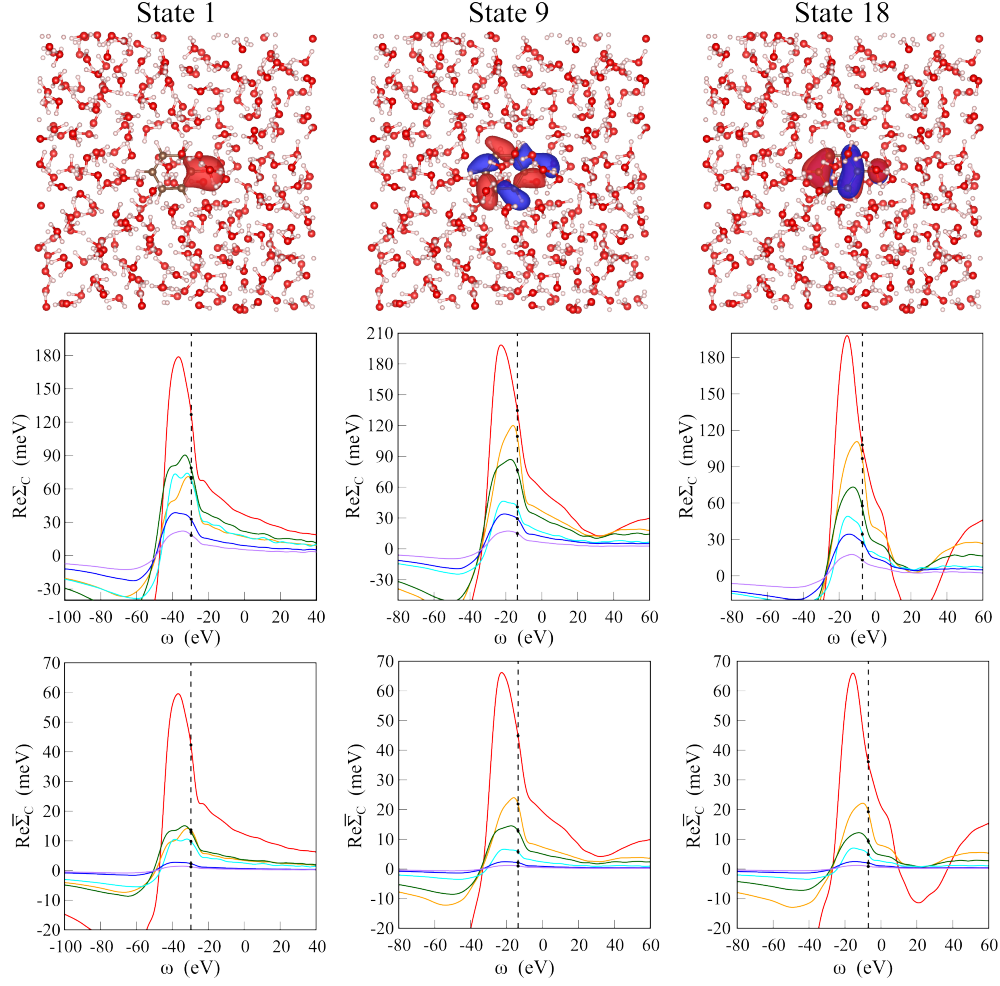

Figure S7: Computational results for phenol in  $\text{H}_2\text{O}$  using the large simulation cell: the 1<sup>st</sup>, 9<sup>th</sup>, and 18<sup>th</sup> ionization states (upper part), real part of the fragment correlation self-energy (before normalization) induced by the corresponding ionization state (middle part), and real part of the fragment correlation self-energy (after normalization) induced by the corresponding ionization state (lower part). The dashed line indicates the QP energy.

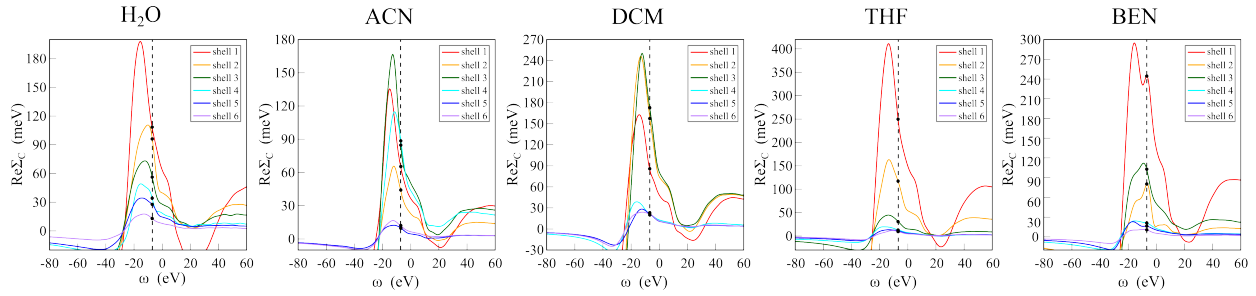

Figure S8: Real part of the fragment correlation self-energy (before normalization) contributed from the six solvation shells of each solvated system. The dashed line indicates the QP energy.

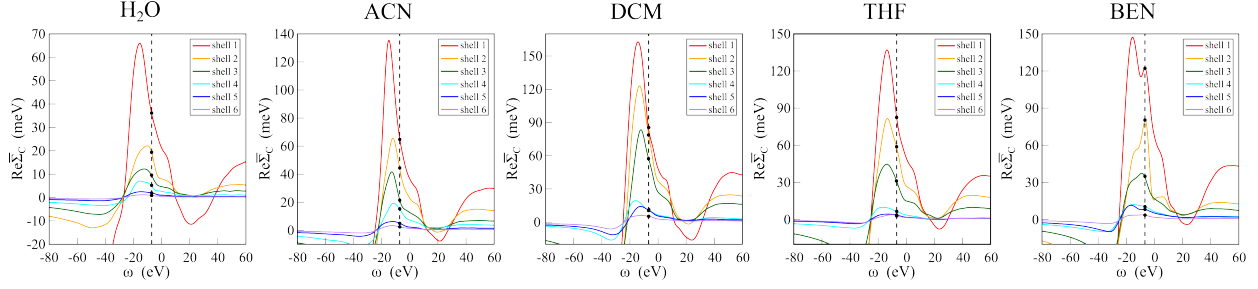

Figure S9: Real part of the fragment correlation self-energy (after normalization) contributed from the six solvation shells of each solvated system. The dashed line indicates the QP energy.

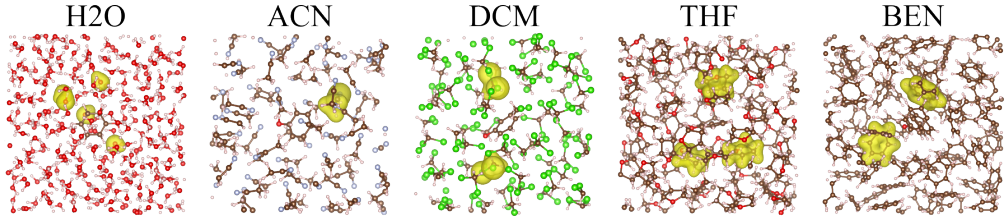

Figure S10: Solvation shells represented by the electron density at  $\sim 5$  Å of each solvated system.

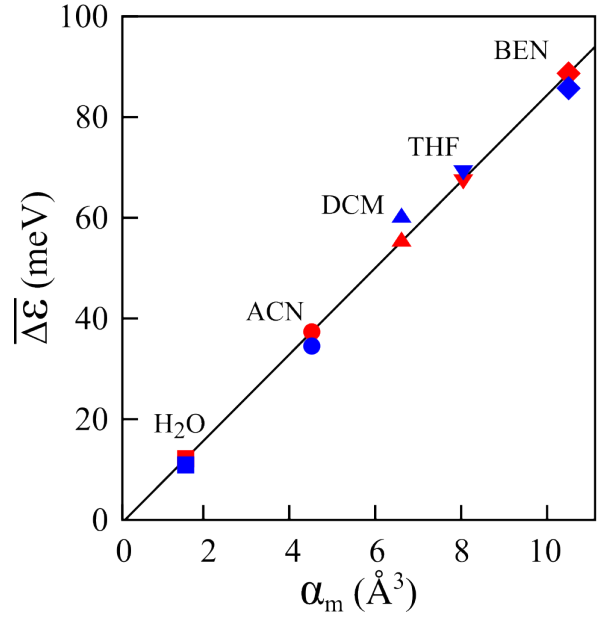

Figure S11: Comparisons between the derived  $\overline{\Delta\epsilon}$  (red) using the straight line and the first-principle ones (blue).

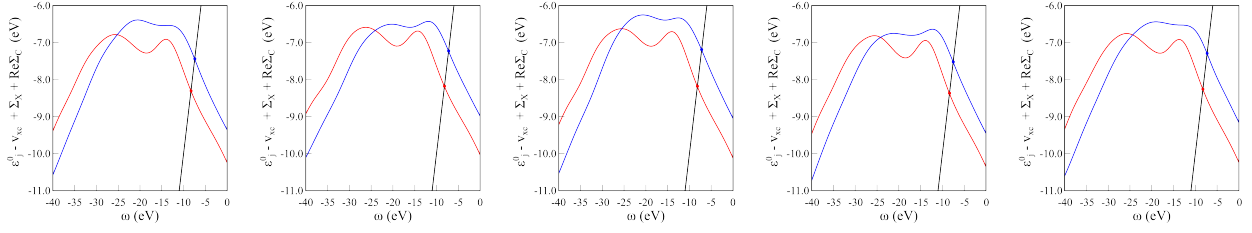

Figure S12: Graphical solutions to the QP energy for phenol in H<sub>2</sub>O using the small simulation cell: the red curve represents the isolated HOMO and the blue curve represents the solvated HOMO. The intersection between each curve and the straight black line indicates the QP energy. Snapshots 1-5 are provided from left to right.

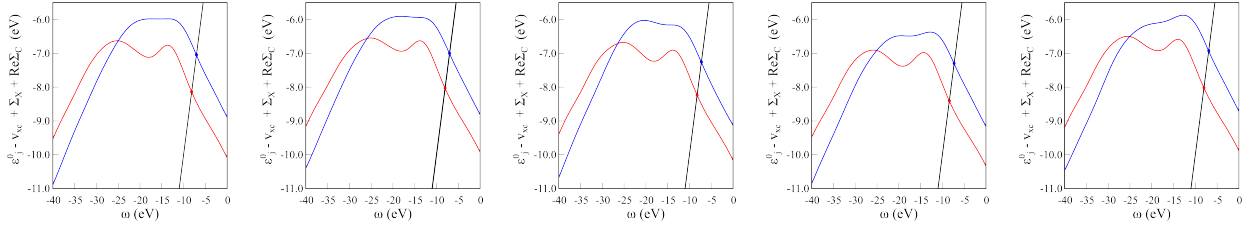

Figure S13: Graphical solutions to the QP energy for phenol in H<sub>2</sub>O using the large simulation cell: the red curve represents the isolated HOMO and the blue curve represents the solvated HOMO. The intersection between each curve and the straight black line indicates the QP energy. Snapshots 1-5 are provided from left to right.

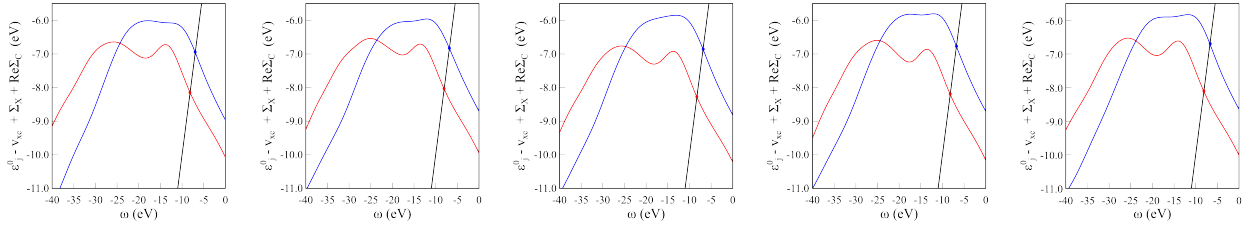

Figure S14: Graphical solutions to the QP energy for phenol in ACN using the small simulation cell: the red curve represents the isolated HOMO and the blue curve represents the solvated HOMO. The intersection between each curve and the straight black line indicates the QP energy. Snapshots 1-5 are provided from left to right.

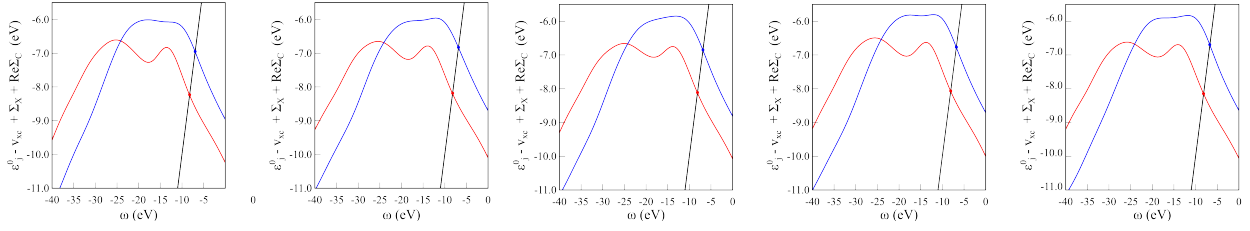

Figure S15: Graphical solutions to the QP energy for phenol in ACN using the large simulation cell: the red curve represents the isolated HOMO and the blue curve represents the solvated HOMO. The intersection between each curve and the straight black line indicates the QP energy. Snapshots 1-5 are provided from left to right.

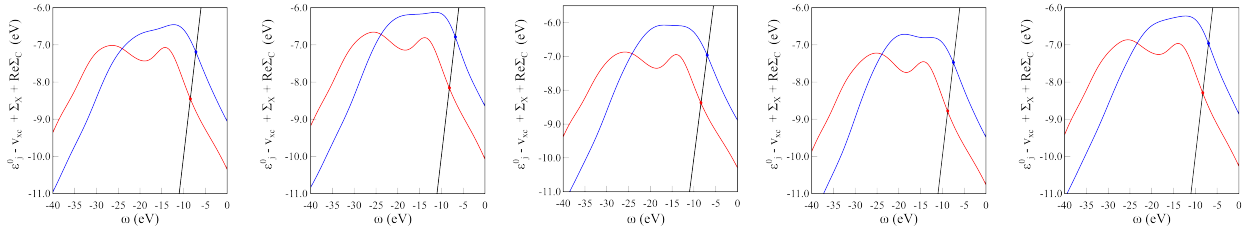

Figure S16: Graphical solutions to the QP energy for phenol in DCM using the small simulation cell: the red curve represents the isolated HOMO and the blue curve represents the solvated HOMO. The intersection between each curve and the straight black line indicates the QP energy. Snapshots 1-5 are provided from left to right.

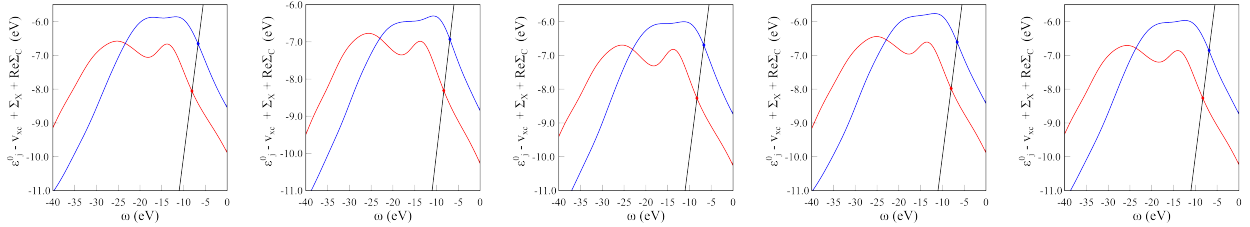

Figure S17: Graphical solutions to the QP energy for phenol in DCM using the large simulation cell: the red curve represents the isolated HOMO and the blue curve represents the solvated HOMO. The intersection between each curve and the straight black line indicates the QP energy. Snapshots 1-5 are provided from left to right.

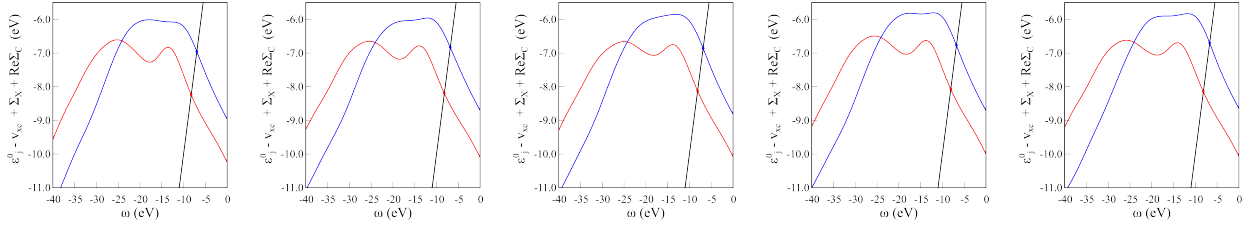

Figure S18: Graphical solutions to the QP energy for phenol in THF using the small simulation cell: the red curve represents the isolated HOMO and the blue curve represents the solvated HOMO. The intersection between each curve and the straight black line indicates the QP energy. Snapshots 1-5 are provided from left to right.

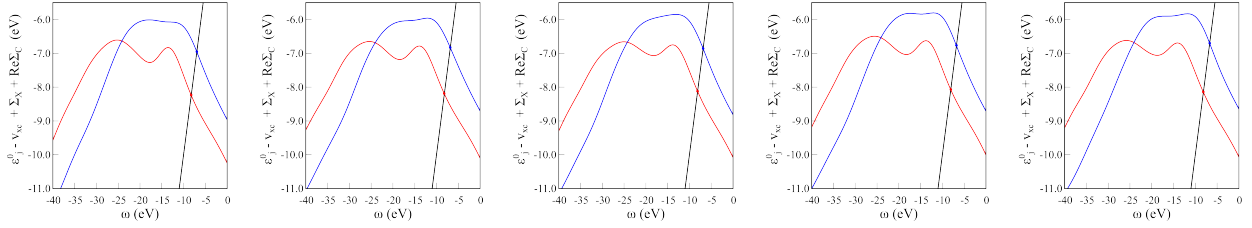

Figure S19: Graphical solutions to the QP energy for phenol in THF using the large simulation cell: the red curve represents the isolated HOMO and the blue curve represents the solvated HOMO. The intersection between each curve and the straight black line indicates the QP energy. Snapshots 1-5 are provided from left to right.

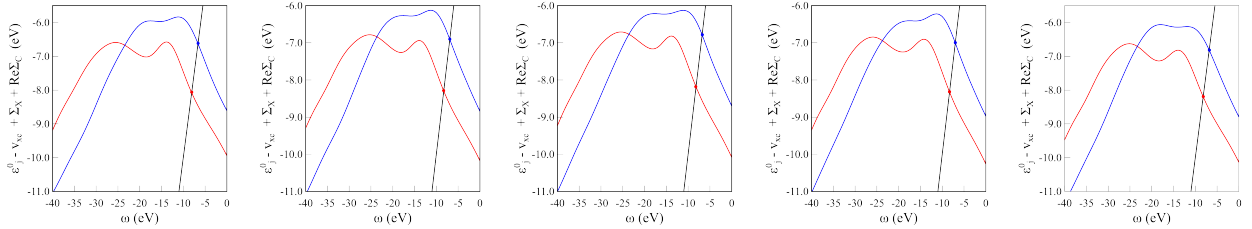

Figure S20: Graphical solutions to the QP energy for phenol in BEN using the small simulation cell: the red curve represents the isolated HOMO and the blue curve represents the solvated HOMO. The intersection between each curve and the straight black line indicates the QP energy. Snapshots 1-5 are provided from left to right.

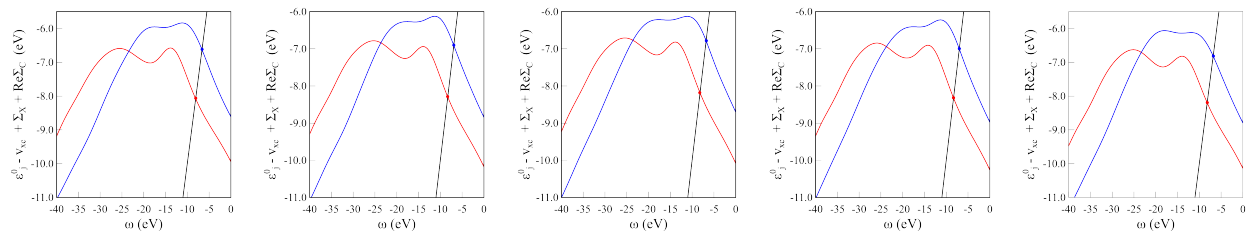

Figure S21: Graphical solutions to the QP energy for phenol in BEN using the large simulation cell: the red curve represents the isolated HOMO and the blue curve represents the solvated HOMO. The intersection between each curve and the straight black line indicates the QP energy. Snapshots 1-5 are provided from left to right.

## References

- (1) Neuhauser, D.; Gao, Y.; Arntsen, C.; Karshenas, C.; Rabani, E.; Baer, R. Breaking the Theoretical Scaling Limit for Predicting Quasiparticle Energies: The Stochastic *GW* Approach. *Physical Review Letters* **2014**, *113*, 076402.
- (2) Vlček, V.; Li, W.; Baer, R.; Rabani, E.; Neuhauser, D. Swift *GW* beyond 10,000 electrons using sparse stochastic compression. *Phys. Rev. B* **2018**, *98*, 075107.
- (3) Vlček, V. Stochastic Vertex Corrections: Linear Scaling Methods for Accurate Quasiparticle Energies. *Journal of Chemical Theory and Computation* **2019**, *15*, 6254–6266.
- (4) Weng, G.; Romanova, M.; Apelian, A.; Song, H.; Vlček, V. Reduced Scaling of Optimal Regional Orbital Localization via Sequential Exhaustion of the Single-Particle Space. *Journal of Chemical Theory and Computation* **2022**, *18*, 4960–4972.
- (5) Berendsen, H. J. C.; van der Spoel, D.; van Drunen, R. GROMACS: A message-passing parallel molecular dynamics implementation. *Computer Physics Communications* **1995**, *91*, 43–56.
- (6) Jorgensen, W. L.; Madura, J. D. Temperature and size dependence for Monte Carlo simulations of TIP4P water. *Molecular Physics* **1985**, *56*, 1381–1392.

- (7) Perdew, J. P.; Burke, K.; Ernzerhof, M. Generalized Gradient Approximation Made Simple. *Phys. Rev. Lett.* **1996**, *77*, 3865–3868.
- (8) Troullier, N.; Martins, J. L. Efficient pseudopotentials for plane-wave calculations. *Phys. Rev. B* **1991**, *43*, 1993–2006.
- (9) Weng, G.; Vlček, V. Efficient treatment of molecular excitations in the liquid phase environment via stochastic many-body theory. *The Journal of Chemical Physics* **2021**, *155*, 054104.
